# Supplementary material for: Medium Amplitude Parallel Superposition (MAPS) Rheology of a Wormlike Micellar Solution
Source: arXiv:2104.11040 ancillary file (2021-04-22)
Supplement: Supplementary file 1 [file WLM_Supplementary.pdf]

Supplementary Material:

# Medium Amplitude Parallel Superposition (MAPS) Rheology of a Wormlike Micellar Solution

Kyle R. Lennon[1], Gareth H. McKinley[2], and James W. Swan[1]

[1]*Department of Chemical Engineering, Massachusetts Institute of Technology, Cambridge, MA 02142*

[2]*Department of Mechanical Engineering, Massachusetts Institute of Technology, Cambridge, MA 02139*

## S1 Derivation of the MAPS Response of the Reptation-Reaction Model

Cates describes a nonlinear viscoelastic model for reversibly breakable polymers [1], such as wormlike micelles, in which the stress tensor is given by:

$$\mathbf{S} = \frac{\beta k_B T}{L_e}\left[\mathbf{W} - \frac{1}{3}\mathbf{I}\right] = \frac{15}{4}G_0\left[\mathbf{W} - \frac{1}{3}\mathbf{I}\right] \tag{S1}$$

with a molecular parameter $\beta$ and an entanglement length $L_e$, together with the thermal energy $k_B T$, defining the elastic modulus $G_0$. The tensor $\mathbf{W}$ is defined by:

$$\mathbf{W} = \int_{-\infty}^{t} \mathcal{B}(v(t')) \exp\left[-\int_{t'}^{t} dt''\mathcal{D}(v(t''))\right] \mathbf{Q}(\mathbf{E}_{t't})dt', \tag{S2}$$

where the tensor $\mathbf{Q}(\mathbf{E}_{t't})$ describes the finite strain deformation in the entangled fluid. This model conceptualizes micelles as polymers diffusing through segments of a constraining tube. These tube segments may be created and destroyed as the individual micelle diffuses, breaks

apart, and recombines. The net rate of tube loss by retraction during a deformation is:

$$v(t) = \mathbf{W}(t) : \mathbf{K}(t), \tag{S3}$$

where $\mathbf{K} = \mathbf{E}_{t't}^{-1} \frac{\partial \mathbf{E}_{t't}}{\partial t}$ is the velocity gradient tensor and $\mathbf{E}_{t't}$ is the deformation tensor. In simple shear:

$$\mathbf{E}_{t't} = \mathbf{I} + \gamma(t, t')\mathbf{e}_1\mathbf{e}_2, \tag{S4}$$

where $\gamma(t', t)$ is the accumulated strain between times $t'$ and $t$, and:

$$\mathbf{K} = \dot{\gamma}(t)\mathbf{e}_1\mathbf{e}_2 = \gamma_0 s(t)\mathbf{e}_1\mathbf{e}_2. \tag{S5}$$

A solution to this modified model can be obtained by first expanding $\mathbf{W}$ as a power series in $\gamma_0$, some characteristic amplitude of the input strain signal:

$$\mathbf{W} = \gamma_0 \mathbf{W}^{(1)} + \gamma_0^2 \mathbf{W}^{(2)} + \gamma_0^3 \mathbf{W}^{(3)} + O(\gamma_0^4). \tag{S6}$$

The resulting expansion of $v(t)$ is:

$$v(t) = \gamma_0^2 W_{12}^{(1)}(t)s(t) + O(\gamma_0^4), \tag{S7}$$

in which we have assumed that the effects of shear stress appear only at odd orders with respect to the input signal. The creation and destruction rates can be similarly written as a power series in $\gamma_0$, with the specification that in the quiescent state both functions are governed by curvilinear diffusion of micelles through tube segment with timescale $\tau$:

$$\mathcal{D} = \frac{1}{\tau} + \left(\frac{d\mathcal{D}}{dv}\right)_{v=0} \gamma_0^2 W_{12}^{(1)}(t)s(t) + O(\gamma_0^4), \tag{S8}$$

$$\mathcal{B} = \frac{1}{\tau} + \left(\frac{d\mathcal{B}}{dv}\right)_{v=0} \gamma_0^2 W_{12}^{(1)}(t)s(t) + O(\gamma_0^4). \tag{S9}$$

Based on the constraint that $\mathcal{D} - \mathcal{B} = v$ [1], we may replace the derivatives of the creation and destruction functions with a single parameter $\alpha$:

$$\alpha \equiv \left(\frac{d\mathcal{D}}{dv}\right)_{v=0} = \left(\frac{d\mathcal{B}}{dv}\right)_{v=0} + 1. \quad \text{(S10)}$$

We can also write the exponential within the expression for $\mathbf{W}$ as a power series:

$$\exp\left[-\int_{t'}^{t} dt'' \left(\frac{1}{\tau} + \alpha\gamma_0^2 W_{12}^{(1)}(t'')s(t'') + O(\gamma_0^4)\right)\right] \approx e^{-(t-t')/\tau}\left(1 - \alpha\gamma_0^2 \int_{t'}^{t} W_{12}^{(1)}(t'')s(t'')dt''\right) + O(\gamma_0^4). \quad \text{(S11)}$$

The tensor-valued function $\mathbf{Q}(\mathbf{E}_{t't})$ possesses a similar expansion (with $\gamma(t',t) = \gamma_0 g(t',t)$). For its shear component:

$$Q_{12} \approx \frac{4}{15}\gamma_0 g(t',t) + d\gamma_0^3 g^3(t',t) + O(\gamma_0^5), \quad \text{(S12)}$$

with $d$ representing a scalar constant (which will be defined shortly). Thus, we can write a polynomial series expression for $\mathbf{W}$ directly from the model equation. The first order term gives:

$$W_{12}^{(1)}(t) = \frac{4}{15}\int_{-\infty}^{t} \frac{1}{\tau} e^{-(t-t')/\tau} g(t',t)dt'. \quad \text{(S13)}$$

This expression resembles the memory kernel $m(t-t') = \frac{\partial G(t-t')}{\partial t'}$ of the familiar single-mode linear Maxwell model. Thus, we find that:

$$G^*(\omega) = \frac{G_0 i\omega\tau}{1 + i\omega\tau}. \quad \text{(S14)}$$

In the weakly nonlinear regime at third order (denoted by the superscript '(3)'), we find that there are three distinct contributions to the shear stress nonlinearity:

$$W_{12}^{(3)} = (\alpha - 1)W_{12,\mathcal{B}}^{(3)} + \alpha W_{12,\mathcal{D}}^{(3)} + W_{12,Q}^{(3)}. \quad \text{(S15)}$$

The first, which arises from a nonlinearity in the creation rate, is (making use of $s(t) = \frac{dg(t)}{dt}$ and $g(t', t) = g(t) - g(t')$):

$$W^{(3)}_{12,\mathcal{B}} = \frac{4}{15}\int_{-\infty}^{t} W^{(1)}_{12}(t')\frac{dg(t')}{dt'}e^{-(t-t')/\tau}g(t', t)dt' \tag{S16}$$

We can write each of the time-dependent functions in terms of their Fourier transforms:

$$W^{(1)}_{12}(t') = \frac{1}{2\pi}\frac{4}{15}\int_{-\infty}^{\infty} e^{i\omega_1 t'}\frac{i\omega_1\tau}{1+i\omega_1\tau}\hat{g}(\omega_1)d\omega_1, \tag{S17}$$

$$\frac{dg(t')}{dt'} = \frac{1}{2\pi}\int_{-\infty}^{\infty} e^{i\omega_2 t'}i\omega_2\hat{g}(\omega_2)d\omega_2, \tag{S18}$$

$$g(t', t) = \frac{1}{2\pi}\int_{-\infty}^{\infty} e^{i\omega_3 t'}\left(e^{i\omega_3(t-t')} - 1\right)\hat{g}(\omega_3)d\omega_3. \tag{S19}$$

This gives:

$$\begin{aligned}
W^{(3)}_{12,\mathcal{B}} &= -\frac{1}{(2\pi)^3}\left(\frac{4}{15}\right)^2\iiint_{-\infty}^{\infty}\frac{\omega_1\omega_2\tau}{1+i\omega_1\tau}\hat{g}(\omega_1)\hat{g}(\omega_2)\hat{g}(\omega_3)d\omega_1 d\omega_2 d\omega_3 \\
&\quad\times\int_{-\infty}^{t} e^{i(\omega_1+\omega_2+\omega_3)t'}\left(e^{i\omega_3(t-t')} - 1\right)e^{-(t-t')/\tau}dt' \\
&= -\frac{1}{(2\pi)^3}\left(\frac{4}{15}\right)^2\iiint_{-\infty}^{\infty}\frac{\omega_1\omega_2\tau}{1+i\omega_1\tau}\hat{g}(\omega_1)\hat{g}(\omega_2)\hat{g}(\omega_3)d\omega_1 d\omega_2 d\omega_3 \\
&\quad\times e^{-t/\tau}\left[\frac{e^{[1/\tau+i(\omega_1+\omega_2)]t'+i\omega_3 t}}{\frac{1}{\tau}+i(\omega_1+\omega_2)} - \frac{e^{[1/\tau+i(\omega_1+\omega_2+\omega_3)]t'}}{\frac{1}{\tau}+i(\omega_1+\omega_2+\omega_3)}\right]_{-\infty}^{t} \\
&= -\frac{1}{(2\pi)^3}\left(\frac{4}{15}\right)^2\iiint_{-\infty}^{\infty}\frac{\omega_1\omega_2\tau}{1+i\omega_1\tau}\hat{g}(\omega_1)\hat{g}(\omega_2)\hat{g}(\omega_3)d\omega_1 d\omega_2 d\omega_3 \\
&\quad\times \tau e^{i(\omega_1+\omega_2+\omega_3)t}\left[\frac{1}{1+i\tau(\omega_1+\omega_2)} - \frac{1}{1+i\tau(\omega_1+\omega_2+\omega_3)}\right].
\end{aligned} \tag{S20}$$

Taking the Fourier transform, we find that the contribution to $G^*_3$ from the creation rate nonlinearity is:

$$G^*_{3,\mathcal{B}}(\omega_1, \omega_2, \omega_3) = -\left(\frac{4}{15}\right)\frac{G_0}{6}\sum_j\sum_{k\neq j}\frac{\omega_j\omega_k\tau^2}{1+i\tau\omega_j}\left[\frac{1}{1+i\tau(\omega_j+\omega_k)} - \frac{1}{1+i\tau\sum_l\omega_l}\right]. \tag{S21}$$

This expression has been symmetrized by the sum over all six permutations of two indices $j$ and $k$ drawn from the set $\{1, 2, 3\}$ of the three frequency arguments, resulting in an additional factor of 1/6 multiplying the summation.

The destruction rate nonlinearity is:

$$\begin{aligned}
W_{12,\mathcal{D}}^{(3)} &= -\frac{4}{15}\int_{-\infty}^{t}\frac{1}{\tau}e^{-(t-t')/\tau}\int_{t'}^{t}W_{12}^{(1)}(t'')\frac{dg(t'')}{dt''}dt''g(t',t)dt' \\
&= \frac{1}{(2\pi)^3}\left(\frac{4}{15}\right)^2\iiint_{-\infty}^{\infty}\frac{\omega_1\omega_2}{1+i\omega_1\tau}\hat{g}(\omega_1)\hat{g}(\omega_2)\hat{g}(\omega_3)d\omega_1 d\omega_2 d\omega_3 \\
&\quad\times\int_{-\infty}^{t}e^{-(t-t')/\tau}e^{i\omega_3 t'}\left(e^{i\omega_3(t-t')}-1\right)dt'\int_{t'}^{t}e^{i(\omega_1+\omega_2)t''}dt'' \\
&= \frac{1}{(2\pi)^3}\left(\frac{4}{15}\right)^2\iiint_{-\infty}^{\infty}\frac{i\omega_1\omega_2}{\omega_1+\omega_2}\frac{1}{1+i\omega_1\tau}\hat{g}(\omega_1)\hat{g}(\omega_2)\hat{g}(\omega_3)d\omega_1 d\omega_2 d\omega_3 \\
&\quad\times\int_{-\infty}^{t}e^{-(t-t')/\tau}\left(e^{i(\omega_1+\omega_2)t'}-e^{i(\omega_1+\omega_2)t}\right)e^{i\omega_3 t'}\left(e^{i\omega_3(t-t')}-1\right)dt'. \qquad \text{(S22)}
\end{aligned}$$

From this expression, we see that the symmetrized contribution to $G_3^*$ is:

$$\begin{aligned}
G_{3,\mathcal{D}}^*(\omega_1,\omega_2,\omega_3) = \left(\frac{4}{15}\right)\frac{G_0}{6}\sum_j\sum_{k\neq j}\frac{i\tau\omega_j\omega_k}{\omega_j+\omega_k}\frac{1}{1+i\tau\omega_j}\Bigg[\frac{1}{1+i\tau(\omega_j+\omega_k)} \\
-\frac{1}{1+i\tau\sum_l\omega_l}+\frac{1}{1+i\tau\omega_{6-j-k}}-1\Bigg]. \qquad \text{(S23)}
\end{aligned}$$

Lastly, the contribution from $\mathbf{Q}$ is:

$$W_{12,Q}^{(3)} = d\int_{-\infty}^{t}\frac{1}{\tau}e^{-(t-t')/\tau}g(t',t)^3dt'. \qquad \text{(S24)}$$

This expression is of the time-strain separable form, thus we see that the contribution to $G_3^*$ is [2]:

$$G_{3,Q}^*(\omega_1,\omega_2,\omega_3) = \frac{15}{4}d\left[G^*(\sum_j\omega_j)-\sum_j G^*(\sum_{k\neq j}\omega_k)+\sum_j G^*(\omega_j)\right]. \qquad \text{(S25)}$$

The final step in the solution is to obtain an expression for the constant $d$ from the full model

formulation. The full expression for the tensor $\mathbf{Q}$ describing the deformation is [1]:

$$\mathbf{Q}(\mathbf{E}_{t't}) = \frac{1}{4\pi}\int_{\mathcal{S}} \frac{[\mathbf{E}_{t't}\cdot\mathbf{u}][\mathbf{E}_{t't}\cdot\mathbf{u}]}{|\mathbf{E}_{t't}\cdot\mathbf{u}|} d^2\mathbf{u}, \tag{S26}$$

with the unit vectors $\mathbf{u}$ integrated over the surface of the unit sphere $\mathcal{S}$. The shear component may be computed by taking the outer product of the first and second elements of the vector $\mathbf{E}_{t't}\cdot\mathbf{u}$:

$$\mathbf{E}_{t't}\cdot\mathbf{u} = (u_1 + \gamma(t',t)u_2)\mathbf{e}_1 + u_2\mathbf{e}_2 + u_3\mathbf{e}_3, \tag{S27}$$

giving,

$$Q_{12} = \frac{1}{4\pi}\int_{\mathcal{S}} \frac{[u_1 + \gamma(t',t)u_2][u_2]}{\sqrt{(u_1+\gamma(t',t)u_2)^2 + u_2^2 + u_3^2}} d^2\mathbf{u}. \tag{S28}$$

In the above expressions, $u_n$ refers to the $\mathbf{e}_n$ component of the unit vector $\mathbf{u}$. It is particularly convenient to integrate in spherical coordinates, with the substitutions:

$$u_1 = \sin\theta\cos\psi, \quad u_2 = \cos\theta, \quad u_3 = \sin\theta\sin\psi, \tag{S29}$$

such that the integral becomes:

$$Q_{12} = \frac{1}{4\pi}\int_0^{\pi}\sin\theta d\theta \int_0^{2\pi} \frac{\sin\theta\cos\theta\cos\psi + \cos^2\theta\gamma(t',t)}{\sqrt{1 + 2\sin\theta\cos\theta\cos\psi + \cos^2\theta\gamma^2(t',t)}} d\psi. \tag{S30}$$

What remains is to expand this integral in powers of $\gamma(t',t)$, and compute the integral. The algebraic manipulations are tedious, however with some simplification we arrive at the previously posed expansion:

$$Q_{12} \approx \frac{4}{15}\gamma(t',t) + d\gamma^3(t',t) + O(\gamma^5(t',t)), \tag{S31}$$

with

$$d = -\frac{4}{105}. \tag{S32}$$

To summarize, the solution for the third order complex modulus in the reptation-reaction model can be represented in three parts:

$$G_3^*(\omega_1,\omega_2,\omega_3) = (\alpha-1)G_{3,\mathcal{B}}^* + \alpha G_{3,\mathcal{D}}^* + G_{3,\boldsymbol{Q}}^* \tag{S33}$$

with:

$$G_{3,\mathcal{B}}^*(\omega_1,\omega_2,\omega_3) = -\left(\frac{4}{15}\right)\frac{G_0}{6}\sum_j\sum_{k\neq j}\frac{\omega_j\omega_k\tau^2}{1+i\tau\omega_j}\left[\frac{1}{1+i\tau(\omega_j+\omega_k)} - \frac{1}{1+i\tau\sum_l\omega_l}\right], \tag{S34}$$

$$\begin{aligned} G_{3,\mathcal{D}}^*(\omega_1,\omega_2,\omega_3) = \left(\frac{4}{15}\right)\frac{G_0}{6}\sum_j\sum_{k\neq j}\frac{i\tau\omega_j\omega_k}{\omega_j+\omega_k}\frac{1}{1+i\tau\omega_j}&\left[\frac{1}{1+i\tau(\omega_j+\omega_k)}\right.\\ &\left. -\frac{1}{1+i\tau\sum_l\omega_l} + \frac{1}{1+i\tau\omega_{6-j-k}} - 1\right], \end{aligned} \tag{S35}$$

and:

$$G_{3,\boldsymbol{Q}}^*(\omega_1,\omega_2,\omega_3) = -\frac{1}{7}\left[G^*(\sum_j\omega_j) - \sum_j G^*(\sum_{k\neq j}\omega_k) + \sum_j G^*(\omega_j)\right]. \tag{S36}$$

## S1.1 Similarity of the MAPS Response of the Corotational Maxwell and RR Models

In the corotational Maxwell model, the polymeric stress is governed by the equation:

$$\frac{1}{\tau}\boldsymbol{\sigma} + \frac{\mathcal{D}\boldsymbol{\sigma}}{\mathcal{D}t} = G_0\dot{\boldsymbol{\gamma}}, \tag{S37}$$

with the velocity profile $\boldsymbol{v}$, rate-of-deformation tensor:

$$\dot{\boldsymbol{\gamma}} = \nabla\boldsymbol{v} + (\nabla\boldsymbol{v})^T, \tag{S38}$$

the corotational derivative:

$$\frac{\mathcal{D}\boldsymbol{\sigma}}{\mathcal{D}t} = \frac{D\boldsymbol{\sigma}}{Dt} + \frac{1}{2}(\boldsymbol{\omega}\cdot\boldsymbol{\sigma} - \boldsymbol{\sigma}\boldsymbol{\omega}), \tag{S39}$$

and the vorticity tensor:

$$\boldsymbol{\omega} = \nabla\boldsymbol{v} - (\nabla\boldsymbol{v})^T. \tag{S40}$$

The MAPS response of the corotational Maxwell model is a special case of the MAPS response of a time-strain separable fluid with a single mode Maxwell linear response [2]:

$$G_1^*(\omega) = \frac{G_0 i\omega\tau}{1 + i\omega\tau}, \tag{S41}$$

$$G_3^*(\omega_1,\omega_2,\omega_3) = A\left[G^*(\sum_j \omega_j) - \sum_j G^*(\sum_{k\neq j}\omega_k) + \sum_j G^*(\omega_j)\right], \tag{S42}$$

with $A = -1/6$. This same expression for time-strain separability was also used to obtain the component $G^*_{3,\boldsymbol{Q}}(\omega_1,\omega_2,\omega_3)$ in the RR model, and it was found that the front-factor for this expression was $-1/7$. This is very close to the front factor for the corotational Maxwell model, and apart from this slight difference in magnitude, the behavior of the third order complex modulus of the corotational Maxwell model and the contribution $G^*_{3,\boldsymbol{Q}}(\omega_1,\omega_2,\omega_3)$ to the third order complex modulus of the RR model are identical. This observation can, in part, explain the relatively close agreement between the experimental MAPS data and the corotational Maxwell model.

# S2 Uncertainty Estimate from Ordinary and Weighted Least Squares

In fitting the linear viscoelastic data in this work to the corotational Maxwell model we employ a least squares regression protocol, and in fitting the experimental MAPS data to

the RR model, we employ a weighted least squares protocol. In both cases, uncertainties in the resulting best fit parameters are computed based on information about the curvature of the (weighted or unweighted) residual sum of squares objective function around the optimum.

In the case of the linear response regression, the sum of squares objective in general has a nonlinear dependence on the model parameters (though the nonlinear dependence is due solely to the parameter $\tau$). However, we may linearize the model (with respect to the parameters) near the optimum, and write the residuals $\boldsymbol{r}$ between the model and data as:

$$\boldsymbol{r}(\boldsymbol{x}) = (\boldsymbol{A}\boldsymbol{x} + \boldsymbol{b}) - \boldsymbol{y}, \tag{S43}$$

with $\boldsymbol{A}$ representing some known values of controlled variables, $\boldsymbol{x}$ representing the model parameters, $\boldsymbol{b}$ representing other known and controlled variables, and $\boldsymbol{y}$ representing the data. In the case of complex-valued data, we simply concatenate the real and imaginary components such that the above formulation is purely real-valued. The residual sum of squares in the neighborhood of the minimum may be approximated by:

$$L(\boldsymbol{x}) = \boldsymbol{r}(\boldsymbol{x})^T \boldsymbol{r}(\boldsymbol{x}). \tag{S44}$$

Thus, in the neighborhood of the optimum, we may treat this problem as linear least squares regression. Assuming Gaussian measurement noise with variance $\sigma^2$, the covariance matrix $\boldsymbol{C}$ of the best fit parameters $\hat{\boldsymbol{x}}$ in this case is related to the Hessian of the objective function:

$$\boldsymbol{C} = (\nabla^2 L)^{-1} \sigma^2, \tag{S45}$$

where $\sigma^2$ may be estimated from the optimal value of the objective:

$$\sigma = \frac{1}{n-m} L(\hat{\boldsymbol{x}}), \tag{S46}$$

where $n$ is the number of data points and $m$ is the number of parameters in the fit. For the linearized problem, the Hessian of the objective is simply:

$$\nabla^2 L = 2\boldsymbol{A}^T\boldsymbol{A}. \tag{S47}$$

Once the Hessian is computed, it can be used to compute the covariance matrix $\boldsymbol{C}$. The diagonal elements of $\boldsymbol{C}$ represent the computed variance of the estimated model parameters $\boldsymbol{x}$: $C_{ii} = \sigma^2_{x_i}$. The uncertainties presented in this work represent the square root of these variances. Thus, to compute the uncertainties in the parameters $G_0$, $\tau$, and $c$, we apply the above approach.

Computing the uncertainties in the weighted least-squares problem is very similar. The sole difference is that the objective function is replaced with the following expression:

$$L(\boldsymbol{x}) = \boldsymbol{r}(\boldsymbol{x})^T\boldsymbol{W}\boldsymbol{r}(\boldsymbol{x}), \tag{S48}$$

for some weighting matrix $\boldsymbol{W}$, which we choose to be the inverse of the covariance matrix of the experimental data. Thus, the Hessian of the objective is now:

$$\nabla^2 L = 2\boldsymbol{A}^T\boldsymbol{W}\boldsymbol{A}. \tag{S49}$$

The remainder of the uncertainty calculation remains the same, with the weighted least squares objective at the optimum now used to estimate $\sigma^2$. The covariance matrix in this case is a $1 \times 1$ matrix, because there is only a single adjustable parameter ($\alpha$). Thus, the sole element of the covariance matrix is the variance in the estimated $\alpha$, and the reported uncertainty for $\alpha$ the square root of this value.

# S3 Predictions of the Giesekus Model

The polymeric stress in the Giesekus model is governed by the following tensorial differential equation:

$$\frac{1}{\tau}\boldsymbol{\sigma} + \boldsymbol{\sigma}_{(1)} + \frac{\alpha}{G_0\tau}\boldsymbol{\sigma}\cdot\boldsymbol{\sigma} = G_0\dot{\boldsymbol{\gamma}}, \tag{S50}$$

where $\boldsymbol{\sigma}_{(1)}$ represents the upper convected derivative:

$$\boldsymbol{\sigma}_{(1)} = \frac{D\boldsymbol{\sigma}}{Dt} - \boldsymbol{\sigma}\cdot\nabla\boldsymbol{v} - (\nabla\boldsymbol{v})^T\cdot\boldsymbol{\sigma}. \tag{S51}$$

The velocity profile is represented here by $\boldsymbol{v}$, and is used to compute the rate-of-deformation tensor:

$$\dot{\boldsymbol{\gamma}} = \nabla\boldsymbol{v} + (\nabla\boldsymbol{v})^T. \tag{S52}$$

The linear response of the Giesekus model is identical to that of the RR model – a single Maxwell mode – and may be similarly combined with a high frequency Rouse contribution. The nonlinear response of the Giesekus model is influenced by the dimensionless parameter $\alpha$, which may take values $\alpha \in [0,1]$ [3]. The MAPS response of the Giesekus model has been previously obtained [2], where the third order complex viscosity is:

$$\frac{\eta_3^*(\omega_1,\omega_2,\omega_3)}{G_0\tau^3} = \frac{\alpha\left((3-2\alpha)+\tau\sum_j\omega_j\right)}{3\left(\prod_j(1+i\tau\omega_j)\right)}\frac{\left(-3-4i\tau\sum_j\omega_j+\tau^2\sum_j\omega_j^2+3\tau^2\sum_j\prod_{k\neq j}\omega_k\right)}{\left(\prod_j(1+i\tau\sum_{k\neq j}\omega_k\right)\left(1+i\tau\sum_j\omega_j\right)}, \tag{S53}$$

and the third order complex modulus may be found by the interconversion expression:

$$G_3^*(\omega_1,\omega_2,\omega_3) = \left(\prod_{m=1}^{3} i\omega_m\right)\eta_3^*(\omega_1,\omega_2,\omega_3). \tag{S54}$$

We fit the predictions of the Giesekus model to the experimental data set using the same weighted least squares objective as described in the main text. As depicted in Figure 6 of the main text, a global minimum in the range $\alpha \in [0,1]$ exists, and the best fit of the Giesekus

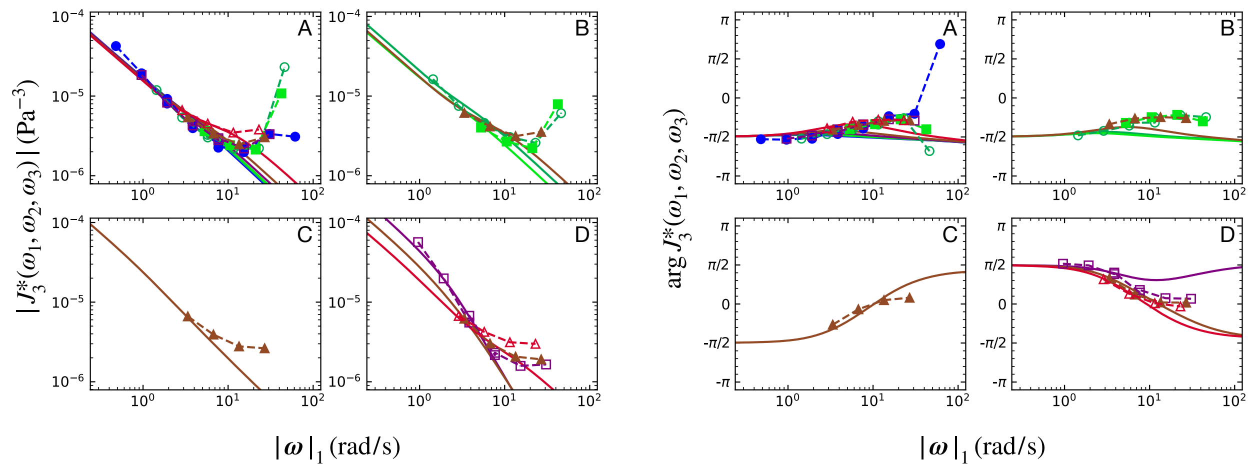


Figure S1: The magnitude (left) and phase angle (right) of the third order complex compliance measured for the wormlike micellar surfactant solution, obtained from a MAPS frequency sweep with $\{n_1, n_2, n_3\} = \{1, 4, 16\}$ over the fundamental frequencies $\omega_0 = 0.16$, 0.32, 0.64, and 1.28 rad/s. Measured data are shown with symbols connected by dashed lines, and predictions of the Giesekus model with $\alpha = 0.9$ are shown with solid lines. Note the systematic deviation at high frequencies.

model to the experimental data occurs with $\hat{\alpha} = 0.9 \pm 0.1$. The predictions of the Giesekus model with $\alpha = 0.9$ are presented alongside the experimental data in Figures S1 and S2. Parity plots of the magnitude and phase angle of the third order complex compliance for the Giesekus model predictions are depicted in Figure S3. As was discussed in the main text, it is clear that there are substantial systematic deviations in the model predictions of both the magnitude and phase of the MAPS response, much more severe than any that occur for predictions of the RR model. As a result, the minimal weighted sum-of-squares error is greater for the Giesekus model than either the RR or corotational Maxwell models.

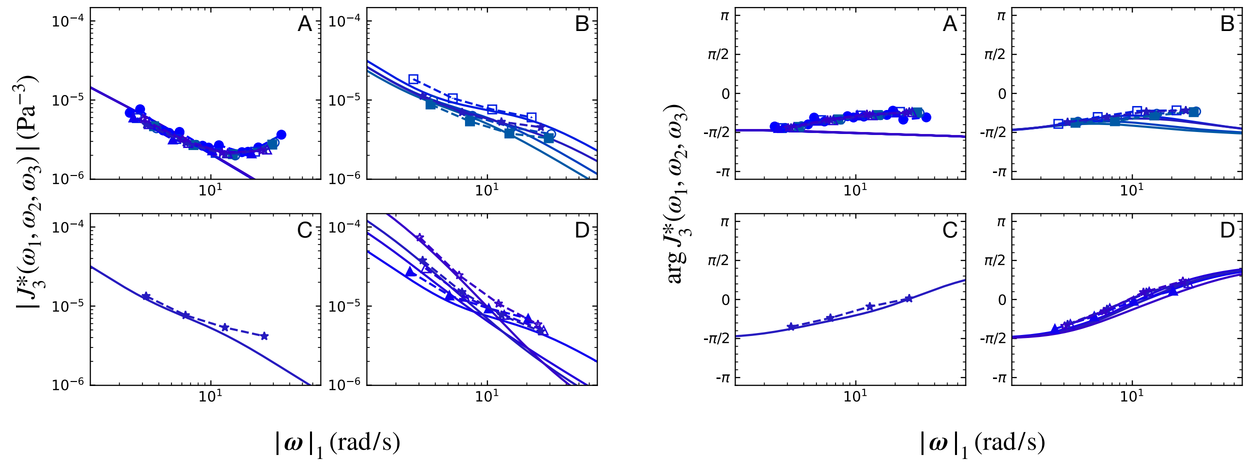


Figure S2: The magnitude (left) and phase angle (right) of the third order complex compliance measured for the wormlike micellar surfactant solution, obtained from a MAPS frequency sweep with $\{n_1, n_2, n_3\} = \{5, 6, 9\}$ over the fundamental frequencies $\omega_0 = 0.16$, 0.32, 0.64, and 1.28 rad/s. Measured data are shown with symbols connected by dashed lines, and predictions of the Giesekus model with $\alpha = 0.9$ are shown with solid lines. Again there are systematic deviations, particularly in subspace A.

# References

[1] M. E. Cates, "Nonlinear viscoelasticity of wormlike micelles (and other reversibly breakable polymers)," *The Journal of Physical Chemistry*, vol. 94, no. 1, pp. 371–375, 1990.

[2] K. R. Lennon, G. H. McKinley, and J. W. Swan, "Medium amplitude parallel superposition (MAPS) rheology. Part 1: Mathematical framework and theoretical examples," *Journal of Rheology*, vol. 64, no. 3, pp. 551–579, 2020.

[3] H. Giesekus, "A simple constitutive equation for polymer fluids based on the concept of deformation-dependent tensorial mobility," *Journal of Non-Newtonian Fluid Mechanics*, vol. 11, no. 1, pp. 69–109, 1982.

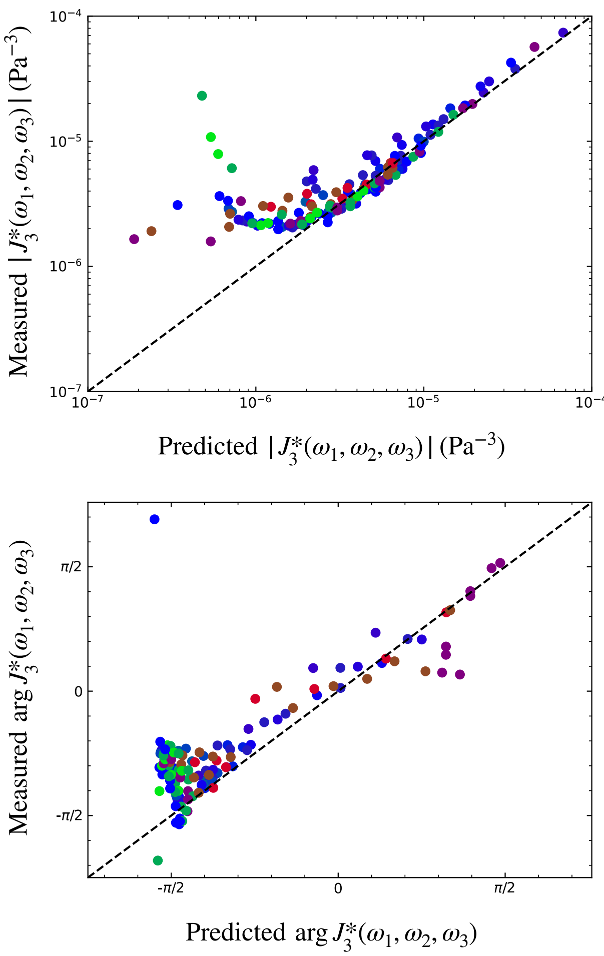


Figure S3: Parity plots of the magnitude (top) and phase angle (bottom) of the third order complex compliance, $J_3^*(\omega_1, \omega_2, \omega_3)$, comparing the values measured by the three-tone MAPS experimental protocol to the values predicted by the Giesekus model with $\alpha = 0.9$. Data from both MAPS frequency sweeps (Figures S1 and S2) are shown on the same axes. Although the agreement may be generally reasonable it is clearly not as good as we can obtain for the RR model, as reflected in the higher weighted mean squared error for the Giesekus model (Figure 6 of the main text).
